# Supplementary material for: Graph Masked Autoencoder for Sequential Recommendation
Source: arXiv:2305.04619 source file (2023-06-01)
Supplement: Supplementary file 1 [file appendix.tex]

\appendix \section{Supplementary Material}
\balance
\label{sec:appendix}
